# Supplementary material for: INFP: Audio-Driven Interactive Head Generation in Dyadic Conversations
Source: arXiv:2412.04037 source file (2024-12-05)
Supplement: Supplementary file 1 [file X_suppl.tex]

% \clearpage
% \setcounter{page}{1}
\maketitlesupplementary

\section{Ablation Study}
We present a visual comparison of two ablation studies.

\textbf{Motion Memory Bank.}
We remove the verbal and non-verbal motion memory banks from interactive motion guider in stage 2, and directly use the dyadic audio feature after several MLP layers as the condition for the motion-attention layer. Results are shown in \cref{fig:mb}. It can be seen that without the memory banks, the generated lip-related motion behaviors are clearly inconsistent with the ground-truth.

\begin{figure}[h]
   \centering
   \includegraphics[width=0.99\linewidth]{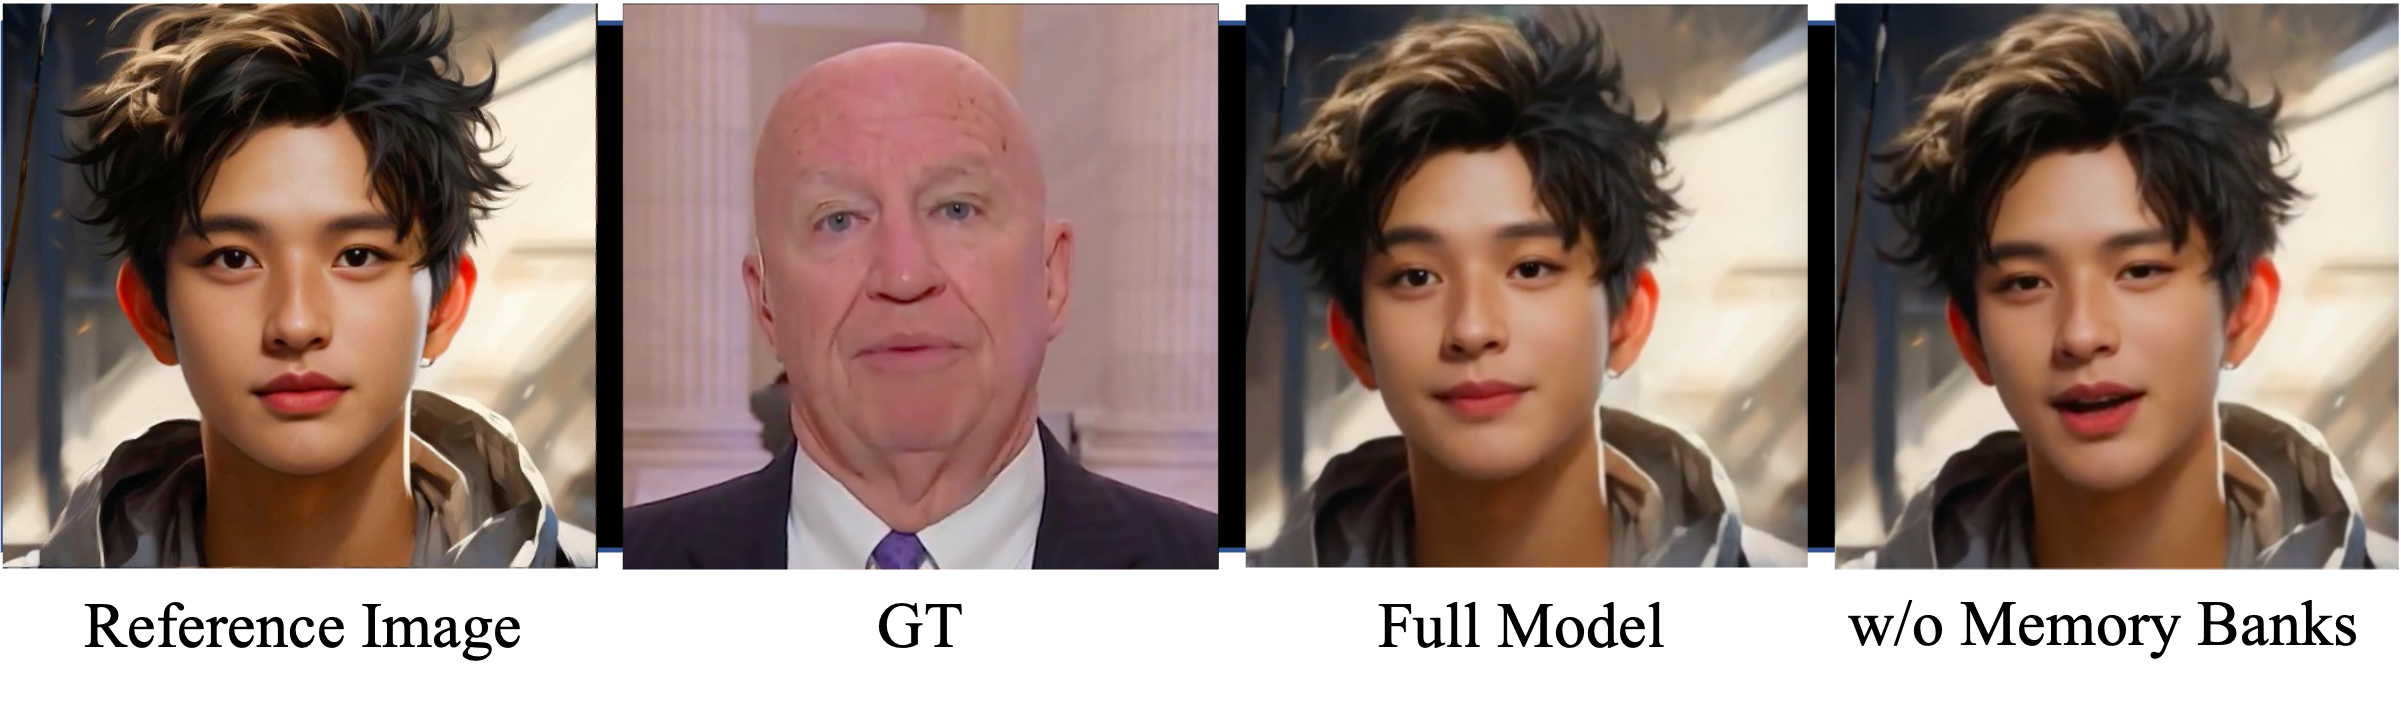}
   \caption{Ablation study on motion memory banks.}
   \label{fig:mb}
\end{figure}

\textbf{Hybrid Facial Representation.} We change the input to $\textbf{E}_{m}$ in stage 1 from our carefully-designed hybrid facial representation to the original intact image or 2D landmarks map. Results are shown in \cref{fig:inp}. It can be seen that there is degradation in generation quality and a leakage of appearance information using original image or landmarks map as input. 

\begin{figure}[h]
   \centering
   \includegraphics[width=0.99\linewidth]{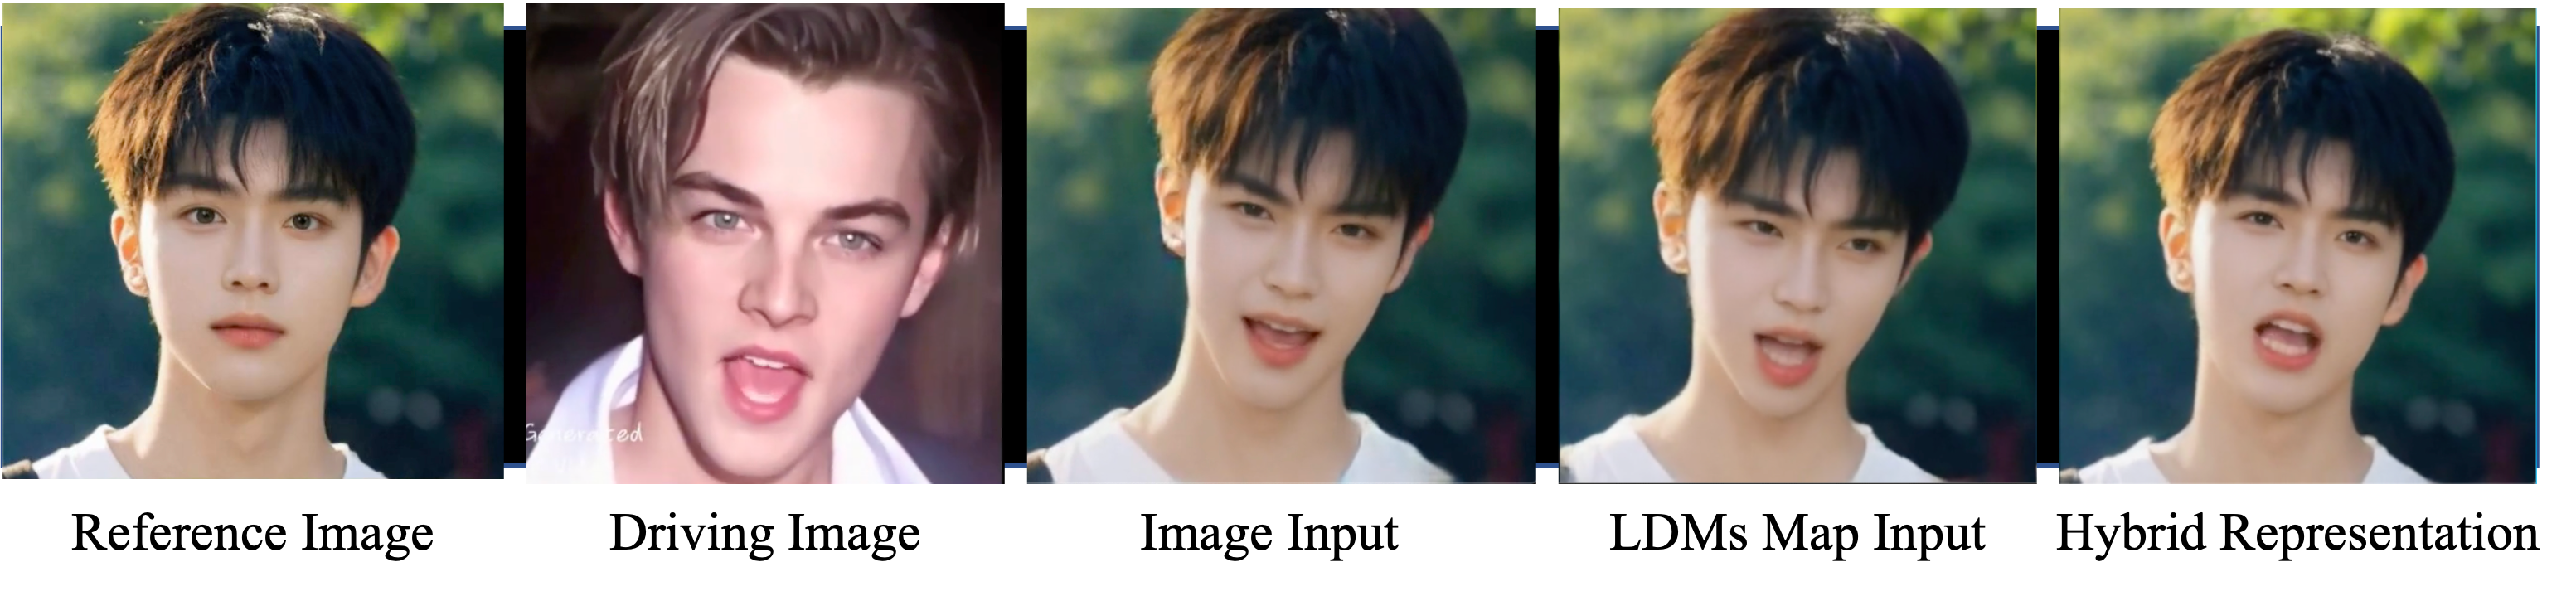}
   \caption{Ablation study on the input to the motion encoder.}
   \label{fig:inp}
\end{figure}

\section{Additional Qualitative Results}
Since our method can naturally generalize to the task of listening head and talking head generation, we directly use our model without any modification to conduct additional experiments.

We first compare our framework with SOTA listening head generation methods, including L2L \cite{ng2022learning}, RLHG \cite{zhou2022responsive} and DIM \cite{DIM}. ViCo \cite{zhou2022responsive} is selected as the benchmark. 
Results are shown in \cref{fig:cmp} (a), which demonstrate that INFP achieves more expressive and diverse motions.

For talking head generation, we select SadTalker\cite{zhang2023sadtalker}, AniTalker\cite{liu2024anitalker}, and EchoMimic\cite{chen2024echomimic} as comparing methods. HDTF \cite{HDTF} is selected as the benchmark.
Results are shown in \cref{fig:cmp} (b), which reveal that INFP can generate more accurate lip movement.

\begin{figure*}[h]
   \centering
   \includegraphics[width=0.7\linewidth]{figs/cmp-t&l-v2.png}
   \caption{Qualitative comparisons with Listening Generation methods (a) and Talking-Head Generation methods (b).}
   \label{fig:cmp}
\end{figure*}

%\section{Failure Cases}
